# Supplementary material for: SOYO: A Tuning-Free Approach for Video Style Morphing via Style-Adaptive Interpolation in Diffusion Models
Source: arXiv:2503.06998 source file (2025-03-10)
Supplement: Supplementary file 1 [file 6_appendix.tex]

\section{Appendix}

\subsection{More details about baselines}\label{sec:baseline_details}
In this section, we provide implementation details for the baseline methods used in our comparative experiments. Each method has been adapted for the video style morphing task according to its characteristics.

\noindent\textbf{{AdaIN~\cite{huang2017arbitrary}}}
For AdaIN adaptation to video style morphing, we first extract the features of both style images using a pre-trained VGG network. Based on the current frame index, we perform spherical interpolation between the VGG features of style A and style B. The interpolated features are then used for Adaptive Instance Normalization with the content frames, enabling a gradual transition between the two styles.

\noindent\textbf{{EFDM~\cite{zhang2022exact}}}
For EFDM, we apply a similar approach as with AdaIN to achieve style morphing. We extract feature representations from both style images and perform spherical interpolation based on the frame index. The interpolated features are then used in EFDM's exact distribution matching process, allowing for a progressive shift between style characteristics while maintaining the method's enhanced style transfer capabilities.

\noindent\textbf{{DiffTuoon~\cite{duan2024diffutoon}}}
Since DiffTuoon is a text-based style transfer method, we adapt it by obtaining textual descriptions of the two style images using GPT-4o~\cite{achiam2023gpt}. These descriptions are converted into embeddings using the model's encoder. We then perform linear interpolation between the two text embeddings based on the frame index being processed. The resulting interpolated embeddings serve as input for the model's encoder hidden states, guiding the diffusion process to create a transition between the described styles.

\noindent\textbf{{StyleID~\cite{chung2024style}}}
For StyleID, we input both style images and perform DDIM inversion on each to obtain their corresponding latent representations $Z_{tA}$ and $Z_{tB}$. We calculate the mean and variance of these representations and perform linear interpolation between them based on the frame index. The interpolated statistics are used for Adaptive Instance Normalization with the content features. For attention-based style injection, we utilize the intermediate attention results from style A for the first half of the video frames and style B for the second half.

\noindent\textbf{{AnyV2V~\cite{ku2024anyv2v}}}
Given that AnyV2V was designed for single-frame editing propagation, we adapt it to the style morphing task by dividing the original video into two equal segments. We apply style transfer with style A for the first half of the video frames and style B for the second half. The final style morphing result is created by concatenating the outputs from both segments, approximating a transition between the two styles.

\subsection{Trade-off between Structure Preservation and Stylization}
In our proposed framework, we inject the query ($Q$) features from the original video throughout the entire denoising process $[0,T]$ to ensure temporal consistency and structural integrity. However, we recognize that in certain artistic applications, users may desire more pronounced stylization effects and are willing to accept a slight compromise in structural fidelity. This represents a fundamental trade-off between structure preservation and stylization degree.

To address this flexibility requirement, we introduce a parameterized injection scheme that allows for controlling the extent of query injection. Specifically, we define a range $[t_{Q_{end}}, T]$ during which the original video's query features are injected. When $t_{Q_{end}} > 0$, we allow the style features to have greater influence on the structural elements of the generated frames during the early denoising stages.

As illustrated in Fig.~\ref{fig:InjectT}, modifying the query injection end point produces varying degrees of stylization. When the injection only occurs within a limited timestep range (e.g., $[0.3T, T]$), the resulting frames exhibit stronger stylistic elements while partially preserving the original structure. Conversely, when the injection spans the entire denoising process $[0, T]$, structural fidelity is maximized but with relatively conservative stylization.

Our experiments reveal that setting the query injection end point to later stages of denoising (e.g., $t_{Q_{end}}=0.1T$ or $t_{Q_{end}}=0.2T$) achieves a favorable balance between structural coherence and stylistic expression. This approach allows for more pronounced style transfer while maintaining sufficient temporal consistency across video frames. However, further increasing the end point (e.g., $t_{Q_{end}}=0.3T$) may introduce structural distortions that compromise video quality.

This parameterization offers users fine-grained control over the stylization-structure trade-off, enabling customization based on specific artistic preferences or application requirements. For applications prioritizing artistic expression, using a higher value for $t_{Q_{end}}$ may be preferable, while applications demanding high temporal consistency should utilize $t_{Q_{end}}=0$ for full range injection.

\begin{figure*}[h]
    \centering
    \includegraphics[width=1\linewidth]{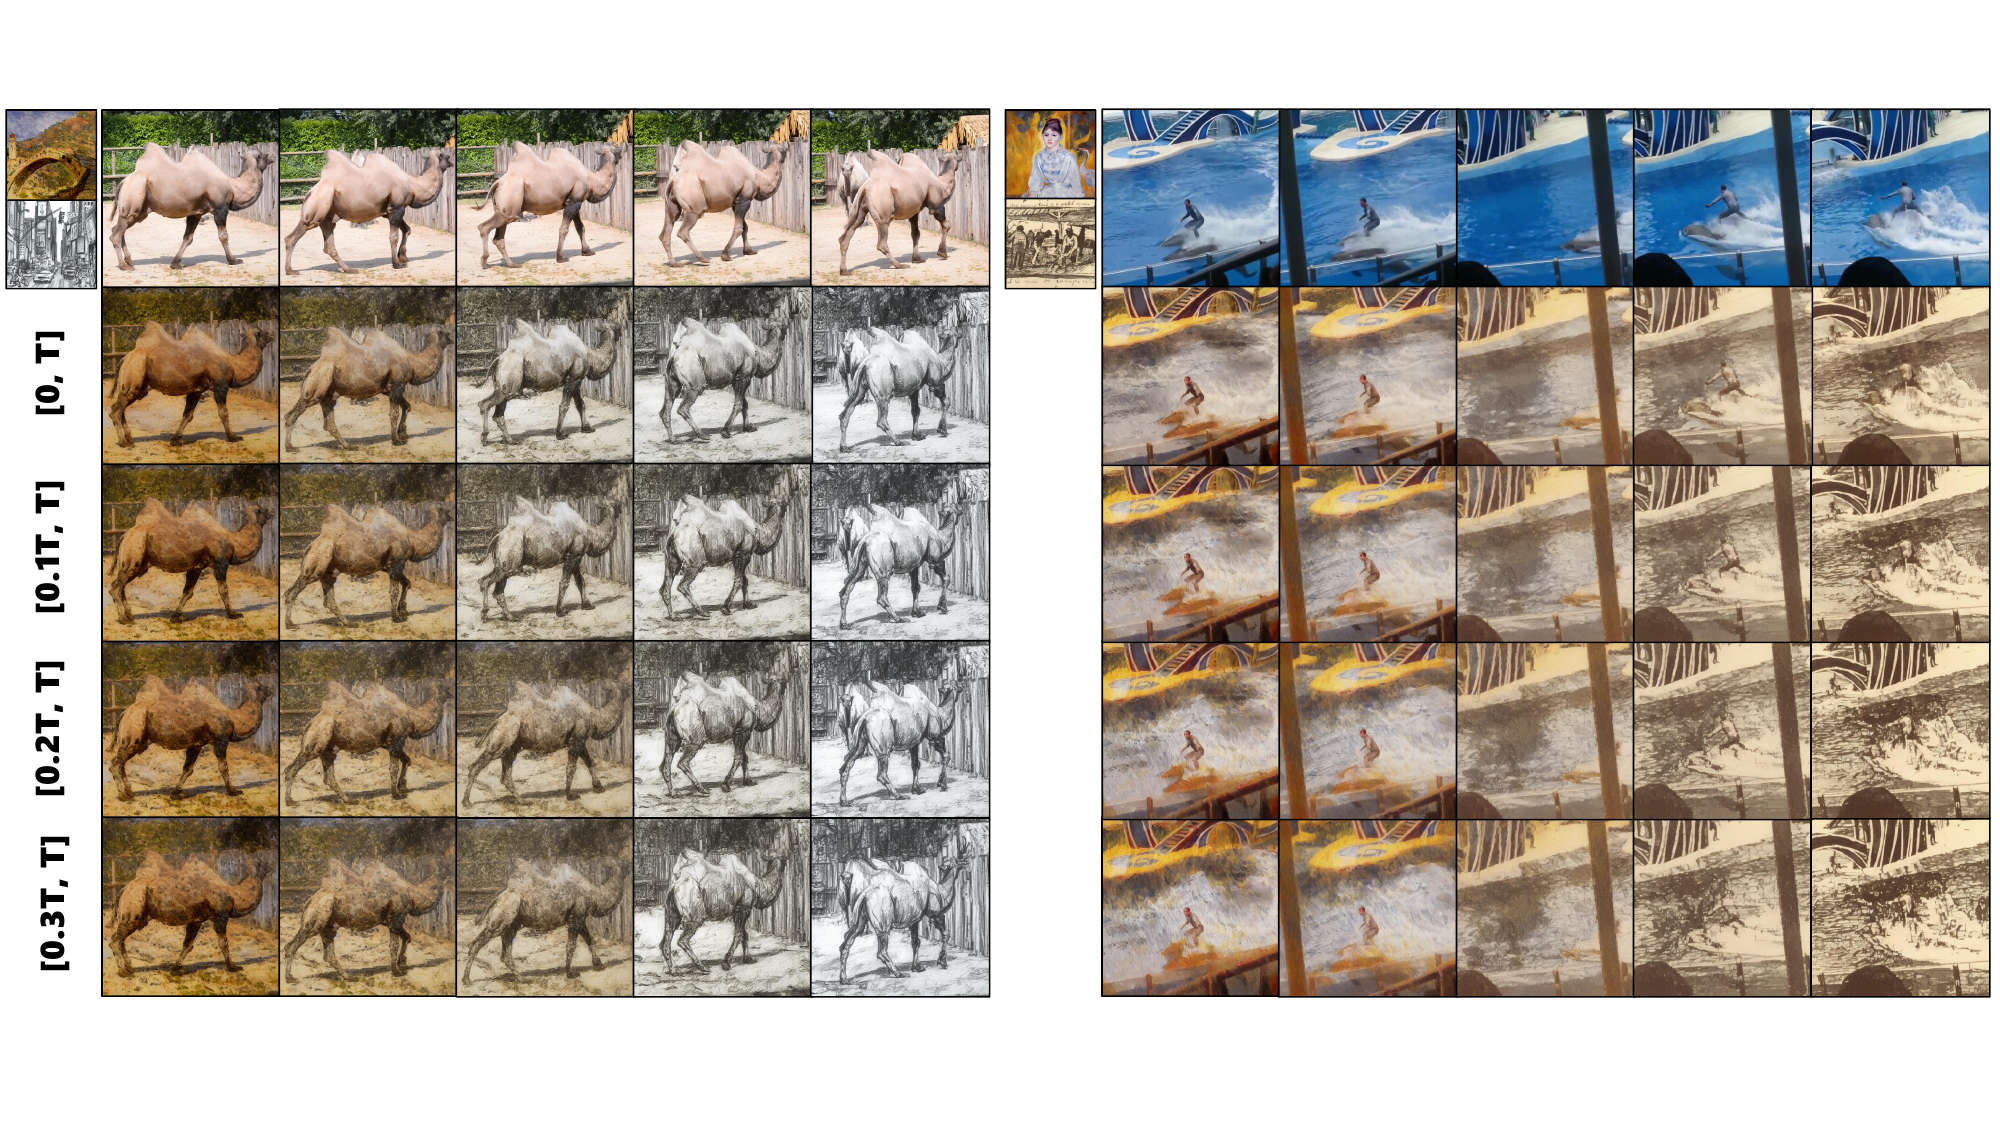} 
    \caption{Visual comparison of stylization effects with different query injection ranges. The top row shows the original video frame and the target style image. Subsequent rows demonstrate the effect of varying $t_{Q_{end}}$ values: when $t_{Q_{end}}=0$, structural integrity is maximized; as $t_{Q_{end}}$ increases (0.1T, 0.2T, 0.3T), stylization becomes progressively more pronounced while gradually compromising structural fidelity, illustrating the trade-off between content preservation and style transfer intensity.}
    \label{fig:InjectT} 
\end{figure*}
